# Supplementary material for: Analysis of conforming, non-matching, and polygonal methods for Darcy and advection-diffusion-reaction simulations in discrete fracture networks
Source: arXiv:1907.12514 source file (2019-07-29)
Supplement: Supplementary file 1 [file Appendix.tex]

\appendix

\section{Virtual element method for DFN} \label{app:vem}

In this part we recall some fundamental aspects of virtual element method for
elliptic problems. For more details refer to
\cite{Ahmad2013,Beirao2016b,Beirao2017,Beirao2017b,BBBPSsupg,BBorth}.

Let us denote by $\mathcal{T}_{\delta,i}$ the polygonal mesh on fracture
$\Omega_i$, for $i \in \{ 1, \ldots, N_\Omega\}$ discrete space for problem
\eqref{eq:darcy_primal_weak_VEM}, built on
$\mathcal{T}_{\delta,i}$:
\begin{gather*}
    V_{\delta,i}=\left\lbrace v\in \mathrm{V}_{i}: v_{|E}\in
    \mathrm{V}_{\delta,i}^E, \forall E \in \mathcal{T}_{\delta,i} \right\rbrace
\end{gather*}
where, for each element $E\in \mathcal{T}_{\delta,i}$ it is
\begin{gather*}
    V_{\delta,i}^E := \{ v\in \mathrm{H}^1(E):\Delta
    v\in\mathbb{P}_n(E),v\in\mathbb{P}_n(e) \,\forall e\subset\partial E, \\
    v_{|\partial E}\in\mathrm{C}^0(\partial E),\, \left(v,p
    \right)_E=\left(\Pi^\nabla_n v,p\right)_E \,\forall
    p\in\mathbb{P}_k(E)/\mathbb{P}_{k-2}(E) \}
\end{gather*}
and $\mathbb{P}_n(\omega)$ is the space of polynomials of maximum order $n$ on $\omega$. The projector
$\Pi^\nabla_n : \mathrm{H}^1(E)\rightarrow \mathbb{P}_n(E)$ is defined as follows:
\begin{gather*}
    \begin{aligned}
        &\left(\nabla\left(v-\Pi_n^\nabla v\right),\nabla p\right)_E=0 \,, &\forall p\in\mathbb{P}_n(E) \\
        &\left(\Pi^\nabla_n v,1\right)_E = \left(v,1\right)_E.
    \end{aligned}
\end{gather*}
Let us denote by $U_{\delta,\Omega_i}$ a finite dimensional subspace of
$U_{\Omega_i}$, then it is possible to re-write problem
\eqref{eq:darcy_primal_weak_VEM} in the finite dimensional spaces: for all for
$i \in \{ 1, \ldots, N_\Omega\}$, find $h_{\delta,i}\in  V_{\delta,i}$ and
$[u]_{\delta,i}\in U_{\delta,\Omega_i}$ such that:
\begin{gather*} %\label{eq:darcy_primal_weak_VEM_discr}
    \begin{aligned}
        &\left(K_i \Pi_{n-1}^0 \nabla h_{\delta,i}, \Pi_{n-1}^0 \nabla
        v_{\delta,i}\right)_{\Omega_i}+S(h_{\delta,i},v_{\delta,i}) = \\
        & \left(f_i,v_{\delta,i}\right)_{\Omega_i}+\sum_{k\in\Gamma_{\Omega_i}}
        \sigma_i(k)\left([u]_{\delta,i,k},v_{\delta,i |\Gamma_k}
        \right)_{\Gamma_k}, &\quad \forall v_{\delta,i} \in V_{\delta,i}\\
        &\sum_{k\in\Gamma_{\Omega_i}}\sigma_i(k) \left( v_{\delta,i |\Gamma_k},
        \psi_{\delta,k} \right)_{\Gamma_k}=0, &\quad \forall \psi_\delta
        \in U_{\delta,\Omega_i}
    \end{aligned}
\end{gather*}
where $\Pi_n^0$ is the element-wise $\mathrm{L}^2$ projection on the space of
polynomials of maximum order $n$, and $S(\cdot,\cdot)$ is any bi-linear form
such that, \cite{Beirao2015b,Beirao2014d}:
\begin{displaymath}
S(v,v)_{|E} \sim  \|\nabla v\|^2_E \quad \forall v\in \ker \Pi^\nabla_n.
\end{displaymath}
